# Supplementary material for: Corex: Pushing the Boundaries of Complex Reasoning through Multi-Model Collaboration
Source: arXiv:2310.00280 source file (2024-08-21)
Supplement: Supplementary file 1 [file eval-details.tex]

\section{Evaluation Details}
\label{appendix:eval-details}

prompts
